# Supplementary material for: LBP: Robust Rate Adaptation Algorithm for SVC Video Streaming
Source: arXiv:1805.00041 source file (2018-06-13)
Supplement: Supplementary file 1 [file appendix_a.tex]

\section{Appendix A}
\begin{lemma}%{Theorem}
Backward algorithm minimizes the number of skips of the current layer and maximizes the number of candidates to the next layer.
\end{lemma}
\begin{proof}
To prove that, without loss of generality, we assume running backward algorithm for base layer decision, and we assume chunk size of 1s. We choose chunk duration of $1s$ just to use more understood deadline formula since dead line of any chunk $i$ is $(i-1)L+d+1$, remember ($s=d+1$), when $L=1s$ this reduces to $i+d$. The proof holds for any chunk duration. According to the backward algorithm, a chunk $i$ is skipped in two scenarios:\\
\begin{itemize}
\item First, when $\sum_{j=1}^{i_s+d}B(j) - \sum_{i\prime>i}\sum_{j=1}^{i_s+d}(x(i\prime,j)) < X_0$. In words, when the the remaining bandwidth is is less than a base layer chunk size. 
Let's first define $\alpha_s=\sum_{j=1}^{i_s+d}B(j)- \sum_{i\prime>i}\sum_{j=1}^{i_s+d}(x(i\prime,j))$. Now let's assume that the remaining size of chunk $i_s$ to be completely fetched  is $\delta_s$, where $\delta_s=X_0-\alpha_s$ 
Let's define the set of all chunks that have indices higher than $i_s$ as $I$. Let's assume that some chunks ${i_1,....,i_n} \in I_s$ where $I_s\subseteq I$ were partially or completely fetched  before $i_s+d$. We first clearly see that skipping any chunk that is not partially or fully fetched before $i_s+d$ ($i \notin I_s$) would not help fetching chunk $i_s$ since $i_s$ need to be fetched before $i_s+d+1$ time slot; it instead increases the number of skips. We prove the second part by contradiction, Now let's assume skipping a chunk $i^\prime$ in $i_1,....,i_n$ will result in less number of skips and higher bandwidth availability for chunks $\{i_s,.....,C\}-\{i\prime\}$ than if $i_s$ was the skipped one. We know that when we skip $i_s$, there will be only one skip among the set $i_s\cup I_s$. However, skipping $i\prime$ would free some bandwidth $B_f$:\\
	(i) if $B_f < \delta_s$, then chunk $i$ still can't be fetched and chunk $i^\prime$ would not be completely fetched within its deadline any more. This would result in 2 skips which contradict the assumption.\\
	(ii) if $B_f \geq \delta_s$, this would lead to fetching chunk $i_s$ and skipping $i^\prime$, so in both cases we would end up having one skip in the set  $i_s\cup I_s$. Since $i^\prime$ offer the same number of skips, we want to see if skipping it would offer higher bandwidth to chunks $\{i_s,.....,C\}-\{i\prime\}$, than what skipping $i_s$ would offer to $\{i_{s+1},.....,C\}$.
	
	First of all, skipping $i_s$ or $i^\prime$ would result in freeing bandwidth of $\alpha_s$.  Skipping $i_s$ would give opportunity to every chunk $i^{\prime\prime}$ in $\{i_{s+1},.....,C\}$ to increase its quality by $\pi_{i^{\prime\prime}}\alpha_s$ where $\pi_{i^{\prime\prime}} \in [0,1]$, and $\sum_{i^{\prime\prime}}\pi_{i^{\prime\prime}}=1$:
	$X(i^{\prime\prime})=\pi_{i^{\prime\prime}}\alpha_s+X_0$\\
	If chunk $i^\prime$ is skipped. $\alpha_s$  may not be completely available to every  $i^{\prime\prime}$ in $\{i_{s},.....,C\}-\{i^{\prime\prime}\}$ since $i^{\prime\prime}$ may have been partially fetched before every $i^{\prime\prime}+d$. If there is non zero $\beta_s(i^{\prime\prime})$ before every $i^{\prime\prime} < i^\prime$, then  
	$X(i^{\prime\prime})=\pi_{i{\prime\prime}}(\sum_{k<i^{\prime\prime}}\beta_s(k))+X_0$\\
	 If skipping $i^{\prime\prime}$ would offer more candidates to higher layer, then () should be higher than () for every $X(i^{\prime\prime})$. However this contradict the fact that 
	 $\pi_{i^{\prime\prime}}(\sum_{k<i^\prime\prime}\beta_s(k)) \leq \pi_{i^{\prime\prime}}\alpha_s$. Therefore, skipping $i_s$ is the optimal choice.

 \item Secondly, when there is a segment of chunks, $I=\{i_s,.....,i_e\}$  with length $l=i_e-i_s+1$, such that:\\
 %$N*L > B_m$, and $((N-1)*L=B_m$
 $\sum_{j=1}^{j=i_e+d}\sum_{i=i_s}^{i_e}x(i,j) = l*X_0$ and $l > B_m$. In words, chunks $i_s$ to $i_e$ need to be in the buffer at a certain time in order to not skip any of them, but their length is larger than the buffer duration. Skipping any of them is fine in term of reducing the number of skips since skipping any of them is one chunk skip. However, for the same reason in (i) skipping $i_s$ is the one that maximizes the number of candidates to the next layer, hence skipping $i_s$ is the optimal choice, and that concludes the proof.
 \end{itemize}
 \end{proof}
 % skipping $i_s$ will result in  which is the first one we show that for maximizing opportunity of getting higher layers of non-skipped chunks, we should skip $i_s$.
%The bandwidth available to each chunk $i\prime \in I - {i_s}$ when chunk $i_s$ is skipped is:\\
%$\sum_{j=1}^{j=i^\prime+d}-sum_{i=}$ where $\delta_1$ is the freed bandwidth when $i_s$ is skipped.
%Now let's suppose, that we skip $i^\prime > i_s$, then the available bandwidth to every $i \in I - {i^\prime}$ is:\\
\section{Appendix B}
\begin{lemma}%{Theorem}
At every layer, forward algorithm finds optimum lower bound on the fetching time of every chunk in which every chunk can't be fetched before no matter how some or all chunk sizes increases beyond the current layer size.
\end{lemma}
\begin{proof}
To prove it, we again assume forward algorithm in base layer decision. First, we assume that after running backward algorithm, we got set $I$ which is the set of chunks that can be fetched. We clearly see that the proof is obvious for Infinite buffer since all chunks in $I$ can be fetched one after another without worrying about buffer overflow and playback time of every chunk. Therefore, if a chunk $i \in I$ is fetched at $X_0$ size , it would be completely downloaded in faster time than if its fetched in size of $X_i > X_0$. Therefore any chunk $j \in I$ would have been fetched in its earliest time if all chunks $i \in I$ and $i < j$ were fetched at base layer quality.

The tricky part is when the buffer is finite, In this case, the buffer  occupancy over time may change, and some time slots that were not used because of buffer overflow in case of fetching base layer may be used if some chunks were fetched in higher sizes since the time when the buffer is full may be different.

Let's assume that the buffer size is $N$ chunks, and $I_s$ is a set contains the indices of the chunks that are in the buffer at time $t_j$.  These chunks could be of same or different sizes such that:
$\sum_{i \in I_s}({\bf 1}(X_i >X_ 0)) + \sum_{i \in I_s}({\bf 1}(X_i >=X_0)) \leq N$
 
Now, let's consider two cases:
\begin{itemize}
\item First, when the buffer is full of base layer chunks at time $t_j$: 

(i) let's assume that chunks in $I_s$ are fetched at base layer size $X_0$ and the playback of the first chunk in the set $i_s$ is equal to $t_j$; otherwise this chunk would have not been chosen to be fetched since it violates the buffer constrain. Remember, the playback of every chunk $i \in I_s$ is $i+d+1$. 

Without loss of generality, let's assume that the chunks that are in the buffer at time $t_j$ are chunks $1$ to $N$, and all chunks after $N$(i.e, $N+1,.....,C$) can be fetched. The total chunks that are buffered at the end of $t_j$ is $N_{t_{j}} \leq N+1-1=N$ and the maximum index of the last chunk that can be fetched at $t_j$ is $N+1$. What would happen is that one chunk would have been played and at most one can be added if the bandwidth at $t_j$ $B(t_j)$ allows since more than 1 chunk would overflow the buffer. Therefore, at the end of the time slot $t_j$ there would be at most N buffered chunks with $N+1$ being the last chunk appended to the buffer. 
 
 (ii) some chunks in $I_s$ are fetched in quality higher than the base layer, $X_i > X_0$ for some $i \in I_s$, then at time $t_j$ the buffer may not be full since fetching higher layers would result in more time per chunk fetching which may lead to less chunks buffered at time $t_j$. Precisely, the number of chunks buffered at time slot $t_j$ is:
 $\sum_{i \in I_s}({\bf 1}(X_i >X_ 0)) + \sum_{i \in I_s}({\bf 1}(X_i >=X_0))=M \leq N$
Note, that the index of the last chunk in the buffer is $M < N$. Let $K=N-M$. Then by the end of $t_j$, the number of chunks at the buffer $N_{t_{j}}  \leq M-1+K+1=N$, since chunk number 1 would have been played, $K+1$ chunks would be the most that can be downloaded at time $t_j$, so the last chunk that can be appended to the buffer at time $t_j$ in order to have full buffer is the chunk $N+1$. Therefore, we just showed that when the buffer is full of base layer chunks at time $t_j$, the earliest time to fetch any chunk can't be before its earliest time if chunks in $I$ are fetched at base layer quality.

 \item Secondly, when the buffer is not full:
 Let's assume the two scenarios again for the same available bandwidth at time $t_j$.\\
 (i) All base layer: in this case there will be $M1$ chunks at base layer quality in the buffer at time $t_j$ ($1,....,M_1$), where $M_1<N$. Let's define $K1$ to be $N-M1$, Then by the end of $t_j$, there will be $N_{t_{j}} \leq M_1-1+K_1+1=N$ chunks at the buffer. Chunk $1$ would have been played back and in order to have N chunks in the buffer, $K+1$ would need to be downloaded at time $t_j$, so chunk $N+1$ would have been the last chunk appended to the buffer.
 (ii)  some chunks in $I_s$ are fetched in quality higher than the base layer, $X_i > X_0$ for some $i \in I_s$, then the number of chunks buffered at time slot $t_j$ is:
 $\sum_{i \in I_s}({\bf 1}(X_i >X_ 0)) + \sum_{i \in I_s}({\bf 1}(X_i >=X_0))=G \leq M_2 < M_1 < N$. Let $K_2=N-M_2$, $K_2 > K_1$. Then by the end of $t_j$, the number of chunks at the buffer $N_{t_{j}}  \leq M_2-1+K_2+1=N$, since chunk number 1 would have been played, then the last chunk that can be appended to the buffer at time $t_j$ in order to have full buffer is the chunk N+1. Therefore, we just showed that when the buffer is full of base layer chunks at time $t_j$, the earliest time to fetch any chunk can't be before its earliest time if all chunks in $I$ are fetched at base layer quality.
 \end{itemize}
 \end{proof}
