# Supplementary material for: LBP: Robust Rate Adaptation Algorithm for SVC Video Streaming
Source: arXiv:1805.00041 source file (2018-06-13)
Supplement: Supplementary file 2 [file appendix_b.tex]

\section{Appendix A: Proof of Lemma 4.1}
According to backward algorithm chunk $i_s$ is skipped in two scenarios:\\
\begin{itemize}
\item First, when:
\begin{equation}
 \sum_{j=1}^{(i_s-1)L+s}B(j) - \sum_{i^\prime>i}\sum_{j=1}^{(i_s-1)L+s}(x(i\prime,j)) < X_0
 \end{equation}
 In words, when the remaining bandwidth is is less than a base layer chunk size. We say remaining bandwidth because backward algorithm starts from back moving toward the first chunk, so priority in bandwidth is given to later chunks.
\item Secondly, when there is a segment of chunks, $I=\{i_s,.....,i_e\}$  with length $N=i_e-i_s+1$, such that:
 %$N*L > B_m$, and $((N-1)*L=B_m$
 \begin{equation}
 \sum_{j=1}^{j=(i_e-1)L+s}\sum_{i=i_s}^{i_e}x(i,j) = N\cdot X_0 \ \text{and} \quad N \cdot L > B_m
 \end{equation}
 In words, chunks $i_s$ to $i_e$ need to be in the buffer at a certain time in order not to skip any of them, but their length is larger than the buffer duration. 
 \end{itemize}
 %Skipping any of them is fine in term of reducing the number of skips since skipping any of them is one chunk skip. %However, for the same reason in (i) skipping $i_s$ is the one that maximizes the number of candidates to the next layer, hence skipping $i_s$ is the optimal choice, and that concludes the proof.
 First of all we clearly see in both scenarios, there should be a skip for a chunk $i$ such that $ i \geq i_s$; otherwise either the buffer or the bandwidth constraint is violated, but the decision is which chunk to skip. It does not need to be skipping $i_s$ in order to satisfy the constraints. However, the skip that maximizes the objective is the optimal choice.
 
 To prove that backward algorithm choice is optimal, Let's assume that there is another algorithm that achieves higher objective by skipping a chunk $i^\prime  > i_s$.
 Since skipping any of them makes the constraints non violated, then the one that maximizes the objective is the optimal choice. The objective function is:
 \begin{equation}
f=\gamma^0\sum_{i=1}^{C}\beta^i Z_{0,i}
\label{equ:eq1_objective}
\end{equation}
Skipping $i_s$ or $i^\prime$ frees bandwidth of $\delta \leq X_0 Mbps$, and since, chunks can't be fetched after their deadlines. The one that have earlier deadline would offer more bandwidth for chunks < $i^\prime$. Mathematically,\\
If $i_s$ frees $\delta=\alpha_1+\gamma_1$, where $\alpha_1$ is the bandwidth that is freed when chunk $i_s$ is skipped for the time period $j \leq deadline(i^\prime-1)$, and $\gamma_1$ is the bandwidth that is freed when chunk $i_s$ is skipped for the time period $j > deadline(i_s-1)$, and If $i^\prime$ frees $\delta=\alpha_2+\gamma_2$, where $\alpha_2$ is the bandwidth that is freed when chunk $i^\prime$ is skipped for the time period $j \leq deadline(i^\prime-1)$, and $\gamma_2$ is the bandwidth that is freed when chunk $i^\prime$ is skipped for the time period $j > deadline(i^\prime-1)$
 
We clearly see since $deadline(i_s) < deadline(i^\prime)$:
\begin{equation}
sum_{i=1}^{i^\prime-1}\beta^i Z_{0,i}+\sum_{i=i_s+1}^{C}\beta^i Z_{0,i})
\label{equ:eq1_objective}
\end{equation}

If $i_s$ is the one that is skipped, then the objective is:
\begin{equation}
f_s=\gamma^0(\sum_{i=1}^{i_s-1}\beta^i Z_{0,i}+\sum_{i=i_s+1}^{C}\beta^i Z_{0,i})
\label{equ:eq1_objective}
\end{equation}

 %later chunks up to either $i^{\prime \prime}$, where $i^{\prime \prime}$ is the the last one before next skip (first case) or $i_e$ (second case) can be fetched and $\delta$ more bandwidth is available, so it can be used to fetch higher layers of chunks $i_s+1$ to $i_m=\min(i_e,i^{\prime \prime})$ and/or basel layer of chunk $i_s-1$. %Therefore, the objective is:

% \begin{equation}
%f=\gamma^0\sum_{i=1}^{i_s-1}\beta^i Z_{0,i}+\gamma^0\sum_{i=i_s+1}^{i_m}\beta^i Y_{0,i}+\gamma^0\sum_{i=m+1}^{C}\beta^i Z_{0,i}+\gamma^1\sum_{i=1}^{C}\beta^i Z_{1,i}+.....+\gamma^n\sum_{i=1}^{C}\beta^i Z_{n,i}
%\label{equ:eq1_objective}
%\end{equation}
 
If $i^\prime > i_s$ is skipped , then the objective is: 
\begin{equation}
f^\prime=\gamma^0(\sum_{i=1}^{i^\prime-1}\beta^i Z_{0,i}+\sum_{i=i^\prime+1}^{C}\beta^i Z_{0,i})
\label{equ:eq1_objective}
\end{equation}

Since $\beta > 1$, we clearly see that $f^\prime$ is less than $f_s$:
\begin{equation}
f^\prime < f_s
\end{equation}
Which contradict the assumption.

\section{Appendix B: Proof of Theorem 4.4}

Since $\gamma \ll 0, \beta > 1$, and $\sum_{j > k}\gamma^j \sum_i\beta^i Z_{j,i} \ll \gamma^k \beta Z_{k,1}$, then, the following holds for any $j > k$:\\

%\begin{equation}
%\gamma^k\beta Z_{k,1} \gg \gamma^j \beta^C Z_{j,C}
%\label{equ:eq1_objective}
%\end{equation}

\begin{equation}
\gamma^k\sum_{i=1}^{C}\beta^i Z_{k,i} \gg \gamma^j\sum_{i=1}^{C}\beta^i Z_{j,i}.
\label{equ:eq1a2}
\end{equation}

(\ref{equ:eq1a2}) implies that the algorithm that delivers more enhancement layers and less base layers can't achieve higher objective. i.e, if there is an algorithm 1 with size decisions ${\mathcal Z}^\prime$, and another one with size decisions ${\mathcal Z}^*$, such taht:\\

%if there is an  algorithm that has higher number of enhancement layers and less number of base layers than what is achieved by backward algorithm on base layer, this algorithm can't have higher objective. i.e, if:\\

\begin{equation}
\sum_{n=1}^N \gamma^n\sum_{i=1}^{C}\beta^i Z_{n,i}^\prime > \sum_{n=1}^N \gamma^n\sum_{i=1}^{C}\beta^i Z_{n,i}^*
\label{equ:eq1_objective}
\end{equation}
and
\begin{equation}
\gamma^0\sum_{i=1}^{C}\beta^i Z_{0,i}^\prime <  \gamma^0\sum_{i=1}^{C}\beta^i Z_{0,i}^*
\label{equ:eq1_objective}
\end{equation}

then:\\

\begin{equation}
\sum_{n=0}^N \gamma^n\sum_{i=1}^{C}\beta^i Z_{n,i}^\prime < \sum_{n=1}^N \gamma^n\sum_{i=1}^{C}\beta^i Z_{n,i}^*
\label{equ:eq1_objective}
\end{equation}

Lemma 4.1 shows that backward algorithm achieves optimal fetching policy when only base layer is considered. Therefore, any algorithm delivers less number of base layer can't have higher objective, so we consider only algorithms that can achieve equal number of base layers to which backward can achieve.
Proposition 1 defines the first time when chunk $i$ can be fetched according to the sizes found by running backward algorithm on base layer.

Now, given the backward decisions of the base layer, the lower bound on the fetching time of the $i$th chunk $(t(i))$, the amount that was scheduled to be fetched for chunk $i$ at time $t(i)$, $(x(i,t(i))$, and the remaining bandwidth at $t(i)$ when backward algorithm was run for base layer decisions ($e(t(i)$), , we define when we skip E1 layer of a chunk.\\
 E1 is skipped in 3 scenarios:
  \begin{itemize}
\item First, when there is a chunk $i_s$ such that its base layer is not fetched, $Z_{0,{i_s}}=0$; otherwise constraint~\ref{equ:c2eq1)} is violated.

\item Secondly, when a chunk $i_s$ was considered as a candidate for base layer quality, but it can't meet its deadline if it is fetched in higher quality:
\begin{equation}
 X_0 < \sum_{j=(t(i_s)+1)}^{(i_s-1)L+s}B(j)+x(i_s,t(i_s))+e(t(i)) - \sum_{i^\prime>i}\sum_{j=t(i)}^{(i_s-1)L+s}(x(i^\prime,j)) < X_1
 \end{equation}
 In words, when the remaining bandwidth is is less than a cumulative E1 size of chunk ($X_1=X_0+Y_1$).
\item Finally, when there is a segment of chunks, $I=\{i_s,.....,i_e\}$  with length $N=i_e-i_s+1$, such that:
 %$N*L > B_m$, and $((N-1)*L=B_m$
 \begin{equation}
 \sum_{j=1}^{j=(i_e-1)L+s}\sum_{i=i_s}^{i_e}x(i,j) = X_1+\sum_{i_s+1}^{i_e} X \ \text{and} \quad N \cdot L > B_m
 \end{equation}
 where $X \in \{X_0,X_1\}$\\
 and\\
  \begin{equation}
 \sum_{j=1}^{j=(i_e-1)L+s}\sum_{i=i_s}^{i_e}x(i,j) = X_0+\sum_{i_s+1}^{i_e} X \ \text{and} \quad N \cdot L \leq B_m
 \end{equation}
 
 In words, chunks $i_s$ to $i_e$, were considered to be fetched at least at base layer quality without violating any of the constraints, but when we run backward algorithm for E1 decisions, we find in order to have some of them at E1 quality, they need to be in the buffer at a certain time, but their total length is longer than the buffer duration.
 \end{itemize}
 %Skipping any of them is fine in term of reducing the number of skips since skipping any of them is one chunk skip. %However, for the same reason in (i) skipping $i_s$ is the one that maximizes the number of candidates to the next layer, hence skipping $i_s$ is the optimal choice, and that concludes the proof.
 For first scenario, any algorithm has to skip E1 of that chunk in order to avoid violating the constraints. For both second and third scenario, we clearly see that there should be a skip for E1 of a chunk $i$ such that $ i \geq i_s$; otherwise either the buffer or the bandwidth constraint is violated, but the decision is which chunk to skip.

 To prove that our Base layer backward followed by forward, and then  E1 backward scan (BL backwrd-forward-E1 Backward)) is optimal for up to E1 layer, Let's assume that there is another algorithm that achieves higher objective by skipping E1 of a chunk $i^\prime  > i_s$.
 Since skipping any of them makes the constraints non violated, then the one that maximizes the objective is the optimal choice. The objective function is:

If we skip E1 of $i_s$ (E1 backward decision), then the objective is:
\begin{eqnarray}
f_s=\sum_{n=0}^1\gamma^n \sum_{i=1}^{i_s-1}\beta^i Z_{n,i}+\gamma^0 \beta^{i_{s}}X_{0}\nonumber \\+\gamma^0 \beta^{i^{\prime}}X_{0}+\gamma^1 \beta^{i^{\prime}}X_{1}+\sum_{n=0}^1\gamma^n \sum_{i=i_s+1\backslash i^\prime}^{C}\beta^i Z_{n,i}.
%\label{equ:eq1_objective}
\end{eqnarray}

If $i^\prime > i_s$ is skipped (any other algorithm), then the objective is: 

\begin{eqnarray}
f^\prime=\sum_{n=0}^1\gamma^n \sum_{i=1}^{i^\prime-1}\beta^i Z_{n,i}+\gamma^0 \beta^{i_{s}}X_{0}\nonumber \\+\gamma^1 \beta^{i_{s}}X_{1}+\gamma^0 \beta^{i^{\prime}}Y_{0}+\sum_{n=0}^1\gamma^n \sum_{i=i^\prime+1}^{C}\beta^i Z_{n,i}.
%\label{equ:eq1_objective}
\end{eqnarray}

Since $\beta > 1$, we clearly see that $f^\prime$ is less than $f_s$:
\begin{equation}
f^\prime < f_s
\end{equation}
Which contradict the assumption.Therefore, Deadline and Buffer Aware Bin Packing algorithm finds optimal policy up to layer E1.
Taking this as base for E2, running backward algorithm at E2 will yield the optimal solution up to E2 since backward yields the optimal solution of the current layer given the lower bound on the fetching time of every chunk, and previous backwar-forward yields the optimal solution of all lower layers. Continuing the same manner up to the $N$th enhancement layer yields the maximum objective, thus solves the original problem optimally. 

%we will see the scenarios when E2 skip is needed. The extra scenario is that when there is a chunk did not get its E1, so it can't get E2 in order to not violate the constraints. Continuing the same manner up to enhancement layer $N$ solves the original problem optimally.

%since $i^\prime$ could be be partially fetched before the deadline of the previous one ($i^\prime -1$), and more of it could be fetched after that. Therefore, the extra bandwidth $\delta$ when this chunk is skipped can't be all used to fetch base and higher layers of chunks with indices less than $i^\prime$. Therefore, If we define the objective when $i_s$ is skipped as $f_s$:
\if 0
\begin{equation}
f_s=\sum_n\gamma^n\sum_{i=1}^{i_s-1}\beta^i Z_{n,i}+\sum_n\gamma^n\sum_{i=i_s+1}^{C}\beta^i Z_{n,i}
\label{equ:eq1_objective}
\end{equation}
and the the objective when $i^\prime$ is skipped as $f^\prime$:
\begin{equation}
f^\prime=\sum_n\gamma^n\sum_{i=1}^{i^\prime-1}\beta^i Z_{n,i}+\sum_n\gamma^n\sum_{i=i^\prime+1}^{C}\beta^i Z_{n,i}
\label{equ:eq1_objective}
\end{equation}
We clearly see that $f^\prime$ is always upped bounded by $f_s$:
\begin{equation}
f^\prime \leq f_s
\end{equation}

\section{Appendix B: Proof of Lemma 2}

To prove it, we again assume forward algorithm in base layer decision. First, we assume that after running backward algorithm, we got set $I$ which is the set of chunks that can be fetched. We clearly see that the proof is obvious for Infinite buffer since all chunks in $I$ can be fetched one after another without worrying about buffer overflow and playback time of every chunk. Therefore, if a chunk $i \in I$ is fetched at $X_0$ size , it would be completely downloaded in faster time than if its fetched in size of $X_i > X_0$. Therefore any chunk $j \in I$ would have been fetched in its earliest time if all chunks $i \in I$ and $i < j$ were fetched at base layer quality.

The tricky part is when the buffer is finite, In this case, the buffer  occupancy over time may change, and some time slots that were not used because of buffer overflow in case of fetching base layer may be used if some chunks were fetched in higher sizes since the time when the buffer is full may be different.

Let's assume that the buffer can have up to $N$ chunks at most, and $I_s$ is a set contains the indices of the chunks that are in the buffer at time $t_j$.  These chunks could be of same or different sizes such that:
$\sum_{i \in I_s}({\bf 1}(X_i =X_ 0)) + \sum_{i \in I_s}({\bf 1}(X_i >X_0)) \leq N$
 
Now, let's consider two cases:
\begin{itemize}
\item First, when the buffer is full of base layer chunks at time $t_j$: 

(i) let's assume that chunks in $I_s$ are fetched at base layer size $X_0$ and the playback of the first chunk in the set $i_s$ is $\geq t_j$. Remember, the playback of every chunk $i \in I_s$ is $(i-1)L+s$. 

Without loss of generality, let's assume that the chunks that are in the buffer at time $t_j$ are chunks $1$ to $N$, and all chunks after $N$(i.e, $N+1,.....,C$) can be fetched. The total chunks that are buffered at the end of $t_j$ is $N_{t_{j}} \leq N+1-1=N$ and the index of the last chunk that can be fetched at $t_j$ is $N+1$. What would happen is that one chunk would have been played and at most one can be added if the bandwidth at $t_j$ $B(t_j)$ allows since more than 1 chunk would overflow the buffer. Therefore, at the end of the time slot $t_j$ there would be at most N buffered chunks with $N+1$ being the last chunk appended to the buffer. 
 
 (ii) some chunks in $I_s$ are fetched in quality higher than the base layer, $X_i > X_0$ for some $i \in I_s$, then at time $t_j$ the buffer may not be full since fetching higher layers would result in more fetching time per chunk which may lead to less chunks buffered at time $t_j$. Precisely, the number of chunks buffered at time slot $t_j$ is:
 $\sum_{i \in I_s}({\bf 1}(X_i >X_ 0)) + \sum_{i \in I_s}({\bf 1}(X_i >=X_0))=M \leq N$.
Note, that the index of the last chunk in the buffer is $M < N$. Let $K=N-M$. Then by the end of $t_j$, the number of chunks at the buffer $N_{t_{j}}  \leq M-1+K+1=N$, since chunk number 1 would have been played, and $K+1$ chunks would be the most that can be downloaded at time $t_j$, so the last chunk that can be appended to the buffer at time $t_j$ in order to have full buffer is the chunk $N+1$. Therefore, we just showed that the earliest time to fetch any chunk can't be before its earliest time if chunks in $I$ are fetched at base layer quality.

 \item Secondly, when the buffer is not full:
 Let's assume the two scenarios again for the same available bandwidth at time $t_j$.\\
 (i) All base layer: in this case there will be $M_1$ chunks at base layer quality in the buffer at time $t_j$ ($1,....,M_1$), where $M_1<N$. Let's define $K_1$ to be $N-M_1$, Then by the end of $t_j$, there will be $N_{t_{j}} \leq M_1-1+K_1+1=N$ chunks at the buffer. Chunk $1$ would have been played back and in order to have N chunks in the buffer, $K+1$ would need to be downloaded at time $t_j$, so chunk $N+1$ would have been the last chunk appended to the buffer.
 (ii)  some chunks in $I_s$ are fetched in quality higher than the base layer, $X_i > X_0$ for some $i \in I_s$, then the number of chunks buffered at time slot $t_j$ is:
 $\sum_{i \in I_s}({\bf 1}(X_i =X_ 0)) + \sum_{i \in I_s}({\bf 1}(X_i >X_0))=G \leq M_2 < M_1 < N$. Let $K_2=N-M_2$, $K_2 > K_1$. Then by the end of $t_j$, the number of chunks at the buffer $N_{t_{j}}  \leq M_2-1+K_2+1=N$, since chunk number 1 would have been played, then the last chunk that can be appended to the buffer at time $t_j$ in order to have full buffer is the chunk N+1. Therefore, we just showed the same result, chunks can't be fetched earlier than if all fetched at base layer.
 \end{itemize}

 \section{Appendix C: Proof of Lemma 3}

First without loss of generality we use chunk duration of $1s$. Therefore, the deadline of any chunk $i$ is $deadline(i)=i+d(i)$ and the playback time of chunk $i$ is $deadline(i)+1$. From lemma 1, we know that when chunks are all fetched in base layer, then every chunk is fetched in its earliest time possible, hence, the minimum stall duration if all chunks are fetched at base layer is the lowest bound to any other fetching policy.
Let's assume that the time slot when chunk $i+1$ is completely fetched is $j$. There are are two scenarios:\\
Scenario 1 ($j \leq deadline(i)+1$): In this case forward algorithm chooses $d(i+1)$ to be equal to $d(i)$ and $deadline(i+1)=i+1+d(i)=deadline(i)+1$, and playback of chunk $i+1$ would be $deadline(i+1)+1=deadline(i)+2$. Since $i+1$th chunk would be completely fetched by the time $deadline(i+1)$, hence there would be no stall, and if the stall duration up to chunk $i$ playback time is  $\alpha$ seconds, then the stall duration up to chunk $i+1$th playback time would be the same ($\alpha$ seconds). Let's assume that there is another algorithm that have $(d(i+1) > d(i))$ and provides same or less stall duration. Let's define $\delta=d(i+1)-d(i)$. Chunk $i$ playback slot is $deadline(i)+1$. Therefore, to avoid any stalls chunk $i+1$ should be played at time slot $deadline(i)+2$. If there is an algorithm such that $(d(i+1) > d(i))$, then chunk $i+1$ playback time would be $deadline(i)+2+\delta$ which has a stall duration of $\delta$ seconds. Therefore, it contradict the assumption that same stall duration can be maintained with $d(i+1) > d(i)$.

Scenario 2 ($j > deadline(i)+1$): then forward algorithm would choose $deadline(i+1)=j$ ($d(i+1)=j-(i+1) > d(i)$) and playback time is $j+1$. Let's re-write it as $d(i+1)=d(i)+\delta$. We clearly see that there would be stall duration of $\delta$ seconds (if chunk $i+1$ is played back at time slot $j+1$) added to the total stall duration up to chunk $i$ which we defined to be $\alpha$ seconds. Therefore, the total stall duration up to playback time of chunk $i+1$ is $(\alpha+\delta)$ seconds. Let's assume that there is an algorithm that have higher deadline ($j^\prime > j$) without introducing more stalls. since chunk $i+1$ is completely fetched at time slot $j$, then the nearest playback time to not introduce more stall duration is to play it back at time slot $j+1$. If it is played at any $j^\prime +1 > j+1$, that would increase the stall duration further and contradict the assumption. This confirms that the forward decision is the optimal in term of minimizing stall duration and concludes the proof.

\fi
